# Supplementary material for: Extended Formulations via Decision Diagrams
Source: arXiv:2211.06065 source file (2023-09-06)
Supplement: Supplementary file 1 [file appendix_experiments.tex]

\section{Details of experiments}
\label{sec:experiments}
\paragraph{Preprocessing of data sets}
The data sets for the $1$-norm regularized soft margin optimization 
are obtained from the libsvm data sets. 
Some of them contain real valued features. We convert real valued features to binary ones 
by rounding them using thresholds specified in Table~\ref{tab:threshold}.  

\begin{table}[h]
    \begin{center}
        \caption{Threshold values used to obtain binary features. The mark ``*'' means the features are already binary.}
         \label{tab:threshold}
        \begin{tabular}{|c||c|} \hline
            Data set   &     Threshold \\ \hline 
            a9a        &   $*$ \\
            art-100000 &   $*$ \\
            %covtype    & $0.5$ \\
            real-sim   & $0.5$ \\
            w8a        &   $*$ \\ 
            %ijcnn12    & $0.5$ \\
            HIGGS      & $0.5$ \\\hline
        \end{tabular}
    \end{center}
  \end{table}

\paragraph{NZDD construction time and summary of data sets}
Computation times for constructing NZDDs for the set covering data sets and soft margin data sets 
are summarized in Table~\ref{tab:nzdd_time_setcover} and \ref{tab:nzdd_time_soft}, respectively. 
Note that the NZDD construction time is not costly and negligible in general 
because once we construct NZDDs, we can re-use those NZDDs for solving optimization problems 
with different objective functions or hyperparameters such as $\nu$ in the soft margin optimization.

\begin{table}[h]
    \begin{center}
        \caption{Computation time for constructing of NZDDs for the set covering.}
         \label{tab:nzdd_time_setcover}
        \begin{tabular}{|c||c|c||c|} \hline
            data set    & zcomp(sec.) & Reducing procedure(sec.) & Total (sec.)\\ \hline 
            connect     &    $0.20$ &    $0.84$ &   $1.04$  \\
            mushroom    &    $0.01$ &    $0.00$ &   $0.01$  \\
            pumsb       &    $1.41$ &    $3.06$ &   $4.47$  \\
            pumsb\_star &    $1.03$ &    $2.40$ &   $3.43$  \\ \hline
            %kosarak     &    $6.07$ &  $455.68$ & $461.75$  \\
            %retail      &    $0.57$ &    $9.28$ &   $9.85$  \\
            %accidents   &    $4.96$ &   $10.73$ &  $15.69$  \\\hline
        \end{tabular}
    \end{center}
\end{table}

\begin{table}[h]
    \begin{center}
        \caption{Computation times for constructing of NZDDs for the soft margin optimization.}
        \label{tab:nzdd_time_soft}
        \begin{tabular}{|c||c|c||c|} \hline
            data set   & zcomp(sec.) & Reducing procedure(sec.) & Total (sec.)\\ \hline 
            a9a        &    $0.04$ &    $0.20$ & $0.24$  \\
            art-100000 &    $0.10$ &    $0.43$ & $0.53$  \\
            % covtype    &    $0.18$ &    $0.00$ & $0.18$  \\
            real-sim   &    $0.24$ &    $0.99$ & $1.23$  \\
            w8a        &    $0.27$ &    $4.20$ & $4.47$  \\ 
            %ijcnn12    &    $0.02$ &    $0.00$ & $0.02$  \\
            HIGGS      &   $13.13$ &    $0.00$ & $13.13$ \\\hline
        \end{tabular}
    \end{center}
  \end{table}
  
  \iffalse
  \begin{table}[htbp]
    \begin{center}
        \caption{maximum memory computation construction of NZDD.}
        % \label{tab}
        \begin{tabular}{|c||c|c||c|} \hline
            data set   & zcmop(megabytes) & Reducing procedure(megabytes) & sum (megabytes)\\ \hline \hline
            a9a        &      $27$ &       $26$ & $53$    \\
            art-100000 &      $33$ &       $41$ & $74$    \\
            % covtype    &      $59$ &        $8$ & $57$    \\
            real-sim   &     $449$ &        $9$ & $458$   \\
            w8a        &      $53$ &       $64$ & $117$   \\ 
            %ijcnn12    &      $25$ &        $8$ & $33$    \\
            HIGGS      &    $1938$ &        $8$ & $1946$  \\\hline
        \end{tabular}
    \end{center}
  \end{table}
\fi

\iffalse
\begin{table}[htbp]
    \begin{center}
        \caption{maximum memory computation construction of NZDD.}
        % \label{tab}
        \begin{tabular}{|c||c|c||c|} \hline
            data set    & zcmop(megabytes) & Reducing procedure(megabytes) & sum (megabytes)\\ \hline \hline
            chess       &    $12$ &     $7$ &    $19$  \\
            connect     &    $37$ &    $50$ &    $87$  \\
            mushroom    &    $13$ &     $4$ &    $17$  \\
            pumsb       &   $179$ &   $322$ &   $501$  \\
            pumsb\_star &   $140$ &   $264$ &   $404$  \\ 
            kosarak     &   $819$ & $42990$ & $43809$  \\
            retail      &   $252$ &  $1218$ &  $1470$  \\
            accidents   &   $307$ &  $1110$ &  $1417$  \\\hline
        \end{tabular}
    \end{center}
\end{table}
\fi

In Table~\ref{tab:summary_setcover} and \ref{tab:summary_soft}, 
we summarize the size of each problem. 
For the set covering problems, the extended formulations have more variables and fewer constraints
as expected. 
For the soft margin optimization problems, 
the extended formulations (\ref{prob:zdd_softmargin_primal2}) have fewer variables and constraints. 
This is not surprising 
since the extended formulation has $O(n+|V|+|E|)$ variables and $O(|E|)$ constraints,  
while the original formulation (\ref{prob:softmargin_primal}) has $O(n+m)$ variables and $O(m)$ constraints.

\begin{table}[h]
    \begin{center}
        \caption{Summary of data sets of the set covering. 
        The term ``original'' and ``extended'' mean the original and the extended formulations, respectively.}
        \label{tab:summary_setcover}
        \begin{tabular}{|c||c|c|c|c||c|c||c|c|c|c|} \hline
            data set    &  \multicolumn{4}{|c|}{Data size} &  \multicolumn{2}{|c|}{Variables} & \multicolumn{2}{|c|}{Constraints}\\ \cline{2-9}
                        &     $n$ &        $m$ &   $|V|$ &    $|E|$ &      Original &   Extended &  Original &   Extended   \\ \hline 
            chess       &    $76$ &     $3196$ &   $219$ &   $1894$ &       $76$ &     $295$ &    $3196$ &   $1896$    \\
            connect     &   $130$ &    $67556$ &  $2827$ &  $25846$ &      $130$ &    $2957$ &   $67556$ &  $25848$    \\
            mushroom    &   $120$ &   $566808$ &    $97$ &    $384$ &      $120$ &     $217$ &  $566808$ &    $386$    \\
            pumsb       &  $7117$ &    $49046$ &   $142$ &  $48199$ &     $7117$ &    $7259$ &   $49046$ &  $48201$    \\
            pumsb\_star &  $7117$ &    $49046$ &   $142$ &  $48199$ &     $7117$ &    $7259$ &   $49046$ &  $48201$ \\ \hline 
           % kosarak     & $41271$ &   $990002$ &  $4507$ & $593661$ &    $41271$ &   $45778$ &  $990002$ & $593663$    \\
           % retail      & $16470$ &    $88162$ &   $120$ &  $83324$ &    $16470$ &   $16590$ &   $88162$ &  $83326$    \\\hline
           % accidents   &   $469$ &   $340183$ &   $103$ & $339683$ &      $469$ &     $572$ &  $340183$ & $339685$    \\\hline
        \end{tabular}
    \end{center}
  \end{table}

\begin{table}[h]
    \begin{center}
        \caption{Summary of data sets of the soft margin optimization.
        The term ``original'' and ``extended'' mean the original and the extended formulations 
        (\ref{prob:softmargin_primal}) and (\ref{prob:zdd_softmargin_primal2}), respectively.}
         \label{tab:summary_soft}
        \begin{tabular}{|c||c|c|c|c||c|c||c|c|c|c|} \hline
            data set   &  \multicolumn{4}{|c|}{Data size} &  \multicolumn{2}{|c|}{Variables} & \multicolumn{2}{|c|}{Constraints}\\ \cline{2-9}
                       &     $n$ &        $m$ &   $|V|$ &    $|E|$ &      Original &  Extended  & Original      & Extended    \\ \hline 
            a9a        &   $123$ &    $32561$ &   $775$ &  $20657$ &    $32685$ &     $21556$ &    $65123$ & $41317$  \\
            art-100000 &    $20$ &   $100000$ &  $4202$ &  $55163$ &   $100021$ &     $59386$ &   $200001$ & $110329$  \\
            % covtype    &    $54$ &    $581012$ &  $129$ &   $1350$ & $581067$   &   $1162025$ &     $1534$ & $2703$ \\
            real-sim   & $20955$ &    $72309$ &    $38$ &   $7922$ &    $93265$ &     $28916$ &   $144619$ &  $15847$  \\
            w8a        &   $300$ &    $49749$ &   $209$ &  $34066$ &    $50050$ &     $34576$ &    $99499$ &  $68135$  \\ 
            ijcnn12    &    $22$ &    $49990$ &     $3$ &     $22$ &    $50013$ &        $48$ &    $99981$ &    $47$  \\
            HIGGS      &    $28$ & $11000000$ &   $151$ &    $989$ & $11000029$ &      $1169$ & $22000001$ &  $1981$  \\\hline
        \end{tabular}
    \end{center}
  \end{table}

\paragraph{Memory consumption}
Figure \ref{fig:memory_setcover}, \ref{fig:memory_soft_artificial}, and \ref{fig:memory_soft_real} 
summarize the maximum memory consumption for the data sets of the set covering, 
synthetic and real data sets of the soft margin optimization, respectively.  
\begin{figure}[h]
    \begin{center}
        \includegraphics[width=8cm,height=4cm,keepaspectratio]{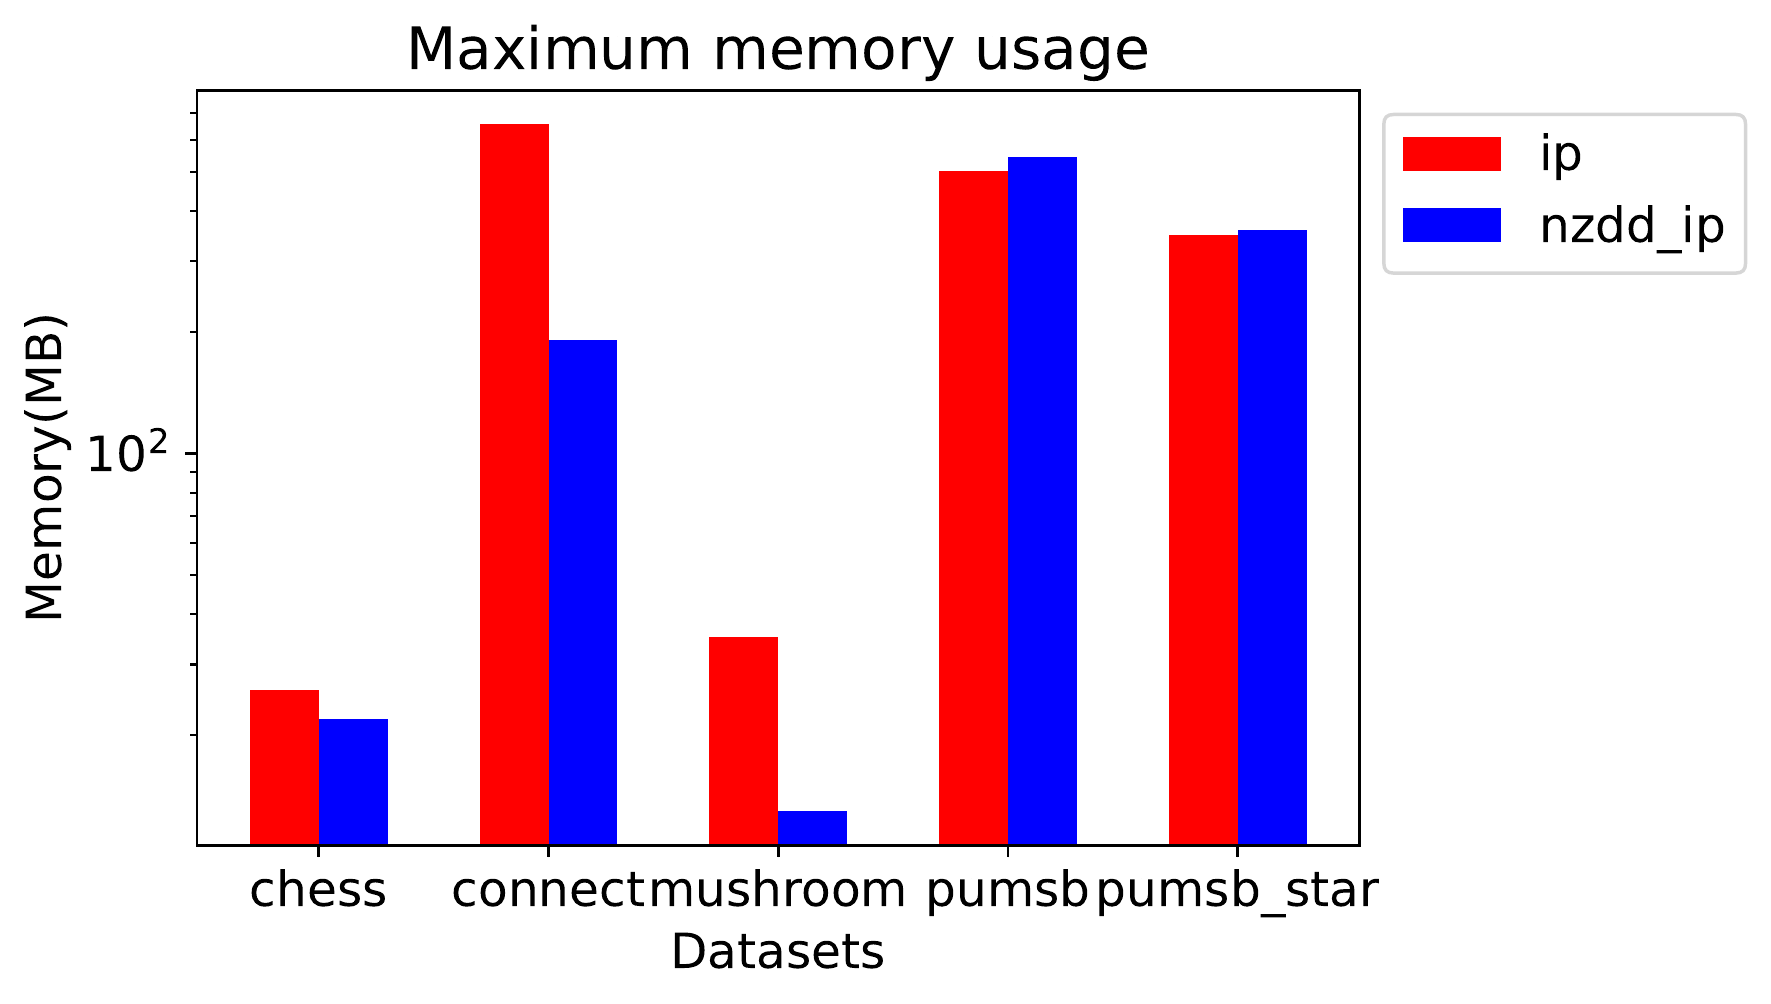}
        \caption{Comparison of maximum memory consumption 
        for real datasets of set covering problems. The y-axes are shown in the logarithmic scale.}
        \label{fig:memory_setcover}   
    \end{center} 
\end{figure}

\begin{figure}[h]
    \begin{center}
        \includegraphics[width=7cm,height=6cm,keepaspectratio]{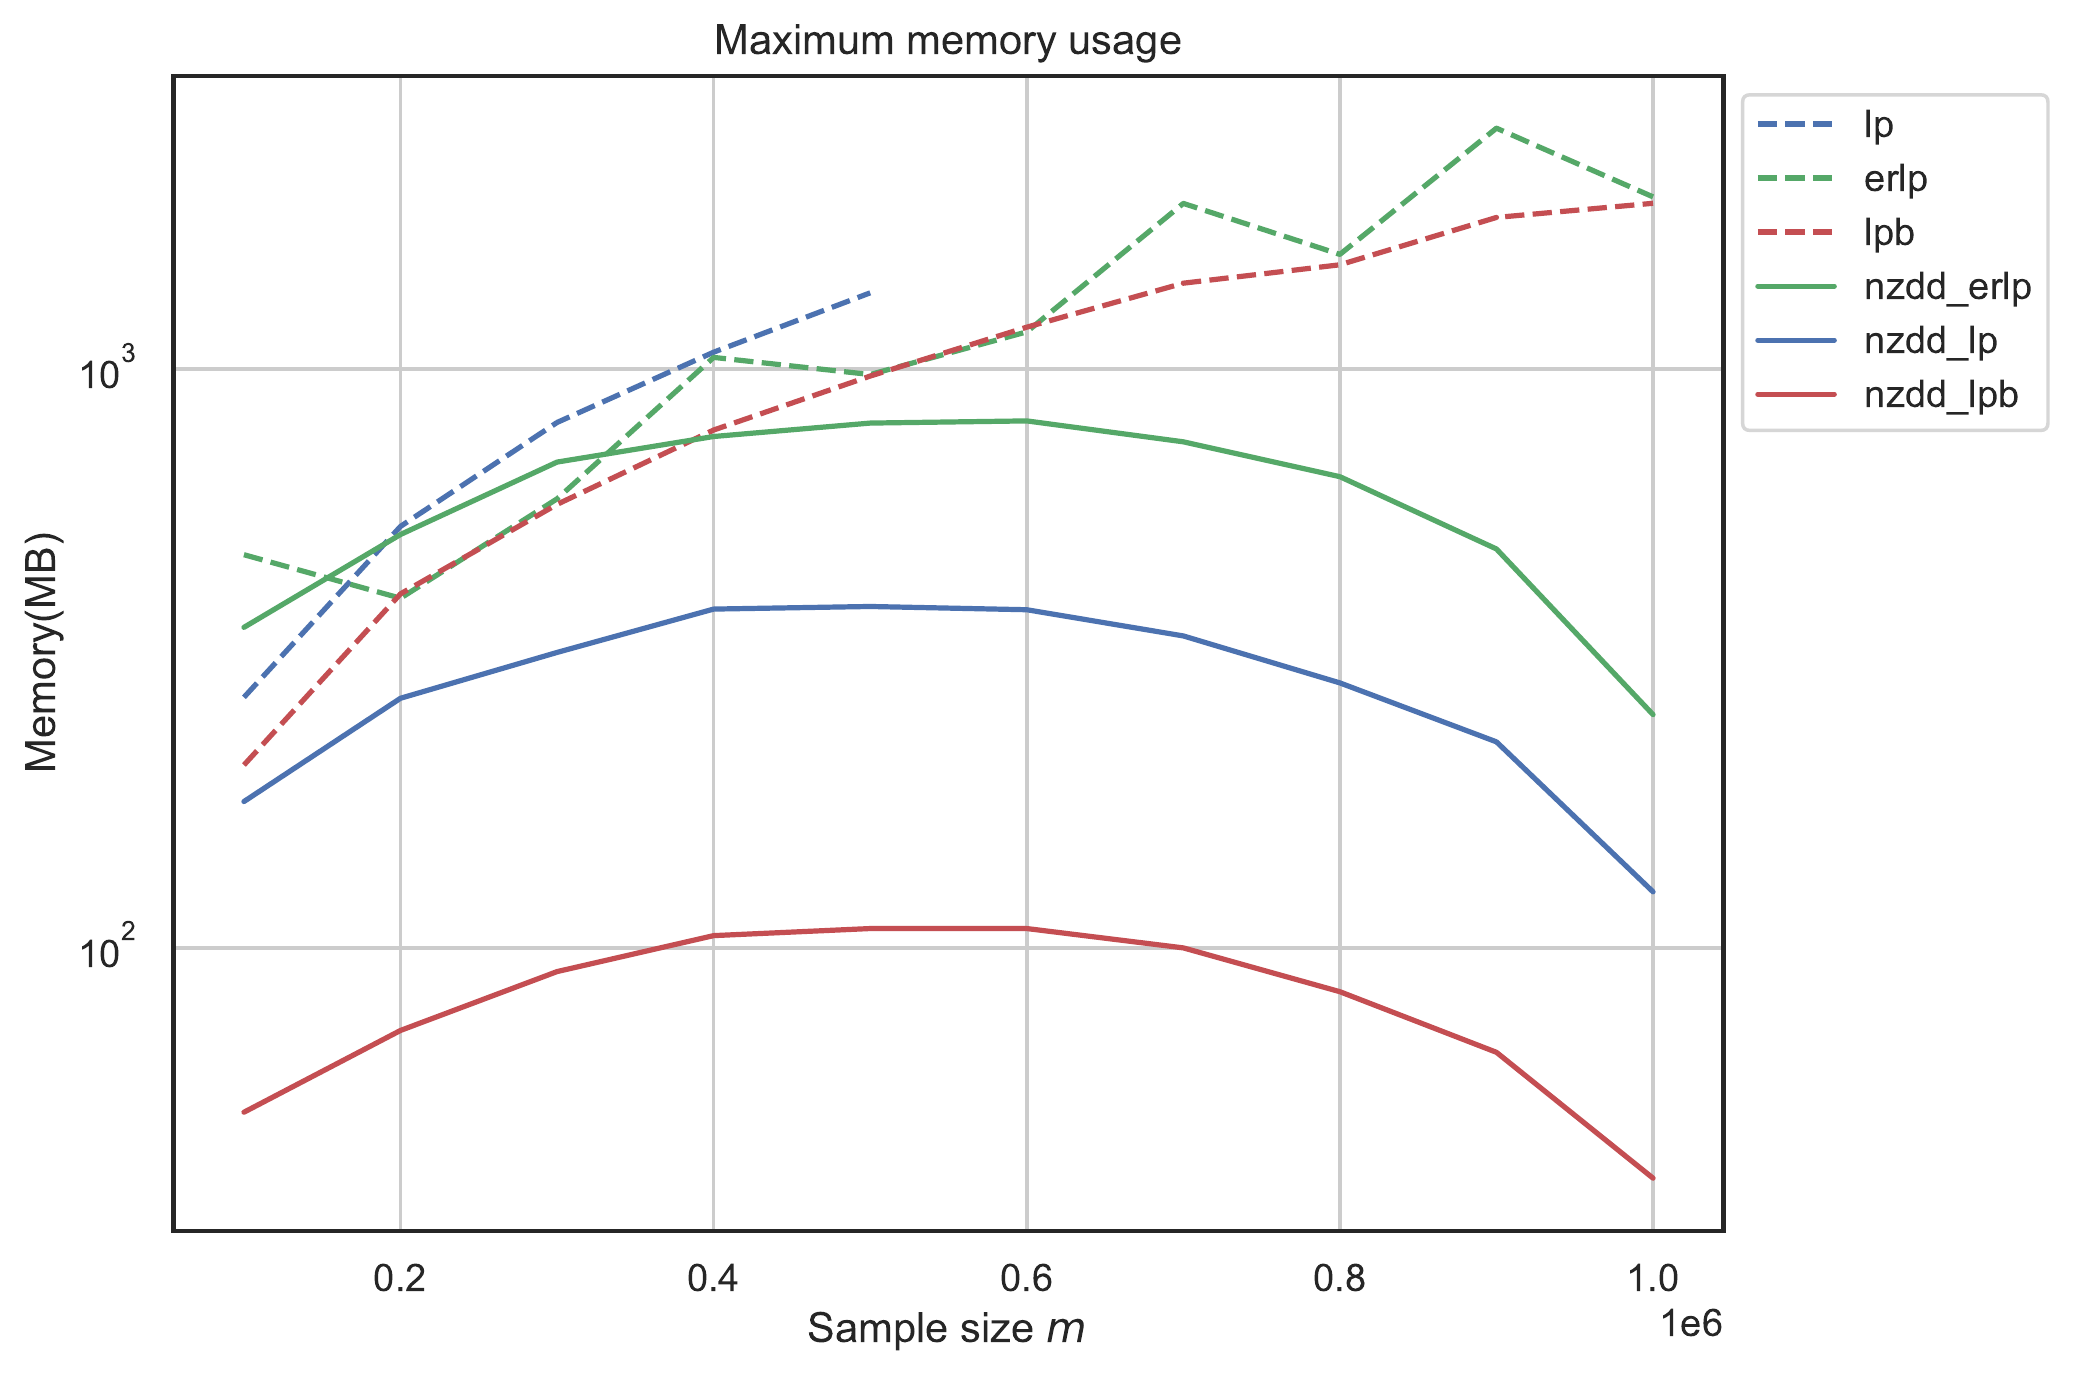}
        \caption{Comparison of maximum memory consumption 
        for synthetic data sets of the soft margin optimization. 
        Results for naive LP w.r.t. $m\geq 6*10^5$ are omitted since it takes more than $1$ day.}
        \label{fig:memory_soft_artificial}
    \end{center}
    
\end{figure}

\begin{figure*}[h]
    \begin{center}
        \includegraphics[width=15cm,height=8cm,keepaspectratio]{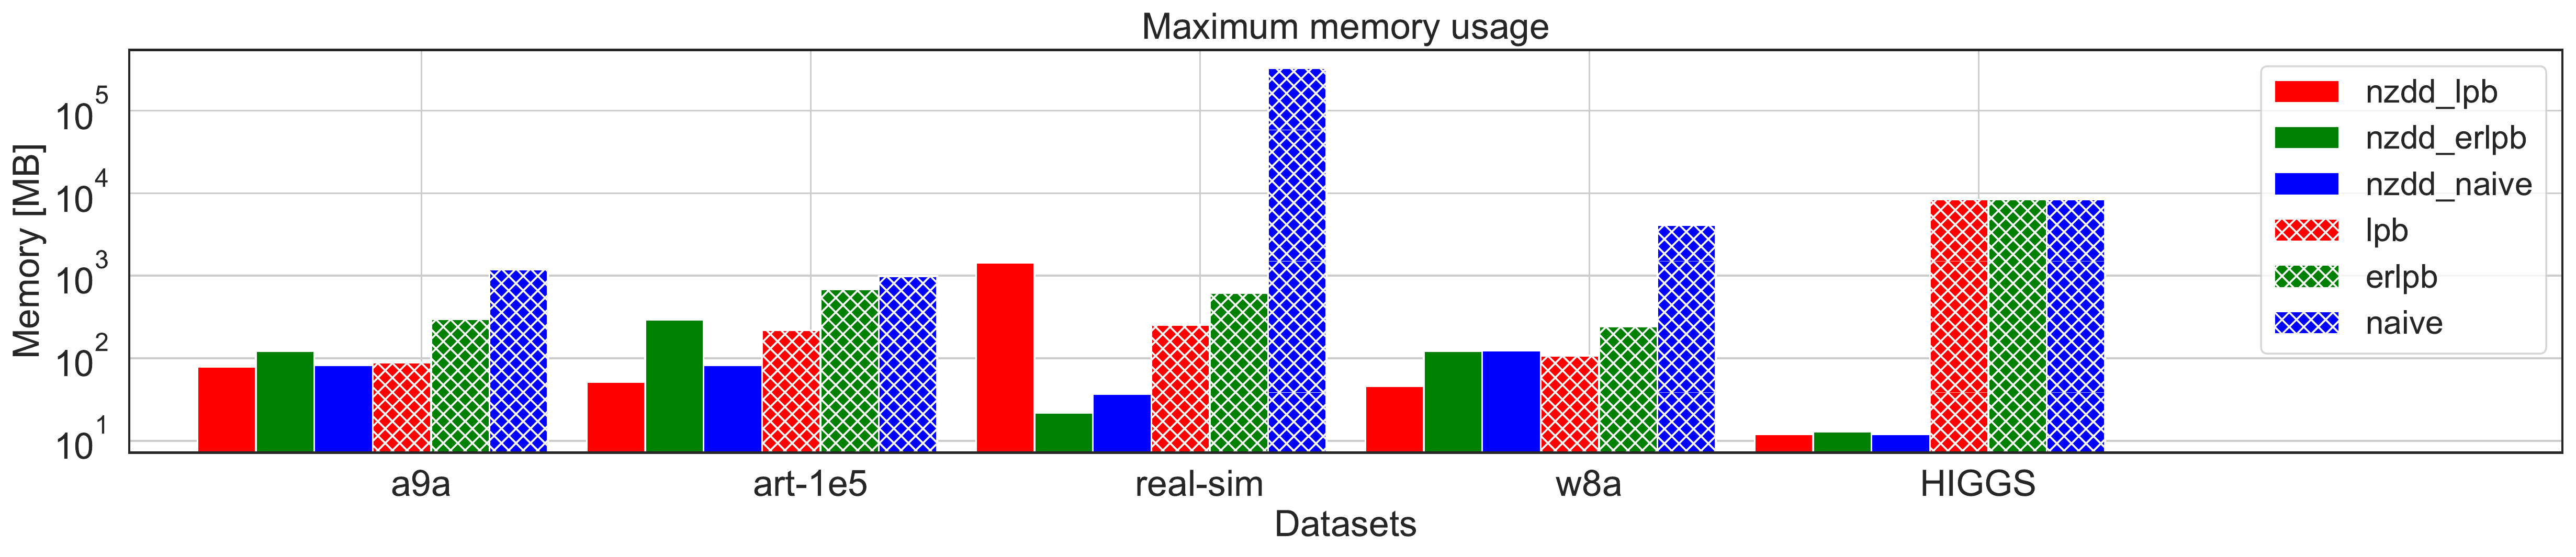}
        \caption{Comparison of maximum memory consumption 
        for real data sets of the soft margin optimization. 
        The y-axes are  plotted in the logarithmic scale.}
        \label{fig:memory_soft_real}
    \end{center}
        
\end{figure*}

\paragraph{Test error rates}
Table~\ref{tab:test_error} summarizes the test error rates of algorithms via the cross validation.
These results imply the extended formulation (\ref{prob:zdd_softmargin_primal2}) is comparable to 
the original problem (\ref{prob:softmargin_primal}) to obtain generalization ability. 
\begin{table}[h]
    \begin{center}
        \caption{Test error rates for real data sets}
        \label{tab:test_error}
        \begin{tabular}{|c|c|c|c|} \hline
            Data sets  & \mytt{lpb} & \mytt{nzdd\_naive} & \mytt{nzdd\_erlp} \\ \hline 
            a9a        & $0.174$ &  $0.159$ & $0.157$ \\
            art-100000 & $0.000$ & $0.0004$ & $0.004$ \\
%                    covtype    & $0.488$ &      $1$ & $0.488$ \\
            real-sim   & $0.179$ &  $0.169$ & $0.532$ \\
            w8a        & $0.030$ &  $0.030$ & $0.029$ \\ \hline
 %           ijcnn12    &         &   $0.09$ &         \\ \hline
        \end{tabular}
    \end{center}
\end{table}

\iffalse
\begin{table}[htbp]
    \begin{center}
        \caption{Comparison of computation times for real data sets.}
        \label{tab10}
        \begin{tabular}{|l||r|r|} \hline
            &\multicolumn{2}{|c|}{Computation time(sec.)} \\ \hline
            data set    & naive LP & proposed\\ \hline
            chess       &     $0.15$ & $0.1$ \\
            connect     &     $7.26$ & $3.82$ \\
            mushroom    &     $0.15$ & $0.01$  \\
            pumsb       &     $14.5$ & $14.23$  \\
            pumsb\_star &    $10.89$ & $8.64$ \\ \hline
        \end{tabular}
    \end{center}
\end{table}

\begin{table}[htbp]
    \begin{center}
        \caption{Comparison of maximum memory consumption for real data sets.}
        \label{tab9}
        \begin{tabular}{|l||r|r|} \hline
            &\multicolumn{2}{|c|}{memory(MB)} \\ \hline
            data set    & naive LP & proposed\\ \hline
            chess       &     $26$ & $22$ \\
            connect     &    $656$ & $192$ \\
            mushroom    &     $35$ & $13$  \\
            pumsb       &    $504$ & $544$  \\
            pumsb\_star &    $348$ & $359$ \\ \hline
        \end{tabular}
    \end{center}
\end{table}
\fi

% pre-processing time of MIP
\begin{table}[h]
    \begin{center}
        \caption{Computation times for constructing of NZDDs for the soft margin optimization.}
        \label{tab:nzdd_time_soft}
        \begin{tabular}{|c||c|c||c|} \hline
            data set   & zcomp(sec.) & Reducing procedure(sec.) & Total (sec.)\\ \hline 
             100000    & 0.08 &  0.14 & 0.22 \\
             200000    & 0.15 &  0.14 & 0.29 \\
             300000    & 0.25 &  0.12 & 0.37 \\
             400000    & 0.31 &  0.08 & 0.39 \\
             500000    & 0.39 &  0.05 & 0.44 \\
             600000    & 0.46 &  0.05 & 0.51 \\
             700000    & 0.53 &  0.03 & 0.56 \\
             800000    &  0.6 &  0.02 & 0.62 \\
             900000    & 0.68 &  0.01 & 0.69 \\
            1000000    & 0.72 &     0 & 0.72 \\\hline
        \end{tabular}
    \end{center}
  \end{table}
