# Supplementary material for: Extended Formulations via Decision Diagrams
Source: arXiv:2211.06065 source file (2023-09-06)
Supplement: Supplementary file 2 [file appendix_softmargin.tex]

\section{Proofs}
In this section, we give some proofs and calculation 
used in the Frank-Wolfe algorithm.
\subsection{Proofs}
\begin{proof}[Proof of lemma~\ref{lem:accuracy_of_theta}]
    Let $F (\bm w, \bm \beta)$ be 
    the objective function of (\ref{eq:smm_on_nzdd}).
    By simple calculation, we can bound $\Theta$ from both sides.
    \begin{align*}
        \Theta(\bm w, \bm \beta)
        & =
        - \frac 1 \eta \ln \frac 1 m
        \sum_{i=1}^{m} \exp
        \left[
            - \eta \left(
                \sign(P_i) \sum_{j \in \Phi(P_i)} w_j
                + \sum_{e \in P_i} \beta_e
            \right)
        \right] 
        - \frac{1}{\nu m} \sum_{e \in E} m_e \beta_e \\
        & \leq
        - \frac 1 \eta \ln \frac 1 m
        \max_{i \in [m]} \exp
        \left[
            - \eta \left(
                \sign(P_i) \sum_{j \in \Phi(P_i)} w_j
                + \sum_{e \in P_i} \beta_e
            \right)
        \right] 
        - \frac{1}{\nu m} \sum_{e \in E} m_e \beta_e \\
        & =
        \min_{i \in [m]}
        \left[
            - \eta \left(
                \sign(P_i) \sum_{j \in \Phi(P_i)} w_j
                + \sum_{e \in P_i} \beta_e
            \right)
        \right] 
        - \frac{1}{\nu m} \sum_{e \in E} m_e \beta_e + \frac 1 \eta \ln m \\
        & = F(\bm w, \bm \beta) + \frac 1 \eta \ln m \\
        \Theta(\bm w, \bm \beta)
        & \geq
        - \frac 1 \eta \ln \max_{i \in [m]} \exp
        \left[
            - \eta \left(
                \sign(P_i) \sum_{j \in \Phi(P_i)} w_j
                + \sum_{e \in P_i} \beta_e
            \right)
        \right] 
        - \frac{1}{\nu m} \sum_{e \in E} m_e \beta_e \\
        & = F(\bm w, \bm \beta)
    \end{align*}
    Therefore, we get
    \begin{align*}
        F(\bm w, \bm \beta) \leq
        \Theta(\bm w, \bm \beta) \leq
        F(\bm w, \bm \beta) + \frac 1 \eta \ln m.
    \end{align*}
    If $(\bm w, \bm \beta)$ is an $\eps/2$-accurate solution 
    and $\eta \geq \frac{2}{\eps} \ln m$, 
    so does an $\eps$-accurate solution of (\ref{eq:smm_on_nzdd}).
\end{proof}

\begin{proof}[Proof of lemma~\ref{lem:smoothness_of_theta}]
    For notational simplicity, we consider the convex function 
    $f: \mathbb R_+^d \to \mathbb R$ defined as
    \begin{align*}
        f(\boldsymbol x) =
        \frac 1 \eta \ln \sum_{i=1}^m e^{- \eta(\bm \alpha_i \cdot \bm x + b_i)},
    \end{align*}
    where $\{ (\bm \alpha_i, b_i) \}_{i=1}^m \subset [-U, U]^d \times \mathbb R$ 
    for some $U > 0$. 
    We prove that $f$ is $2U^2 \eta$-smooth w.r.t. $\ell_1$-norm.
    First of all, we can write the gradient vector and Hessian as
    \begin{align*}
        \nabla f(\bm x) 
        &= - \sum_{i=1}^n \bm \alpha_i p_i(\bm x) \in [-U, U]^d \\
        \nabla^2 f(\bm x)
        &= \eta \sum_{i=1}^n \bm \alpha_i \bm \alpha_i^\top p_i(\bm x)
        + \nabla f(\bm x) \nabla f(\bm x)^\top,
    \end{align*}
    where 
    \begin{align*}
        p_i(\bm x) =
        \frac{e^{-\eta (\bm \alpha_i \cdot \bm x + b_i)}}
             {\sum_{k=1}^n e^{-\eta (\bm \alpha_{k} \cdot \bm x + b_{k})}}.
    \end{align*}
    We can bound the quadratic form as
    \begin{align*}
        \forall \bm x \in \mathbb R_+^d, \quad
        \bm x^\top \nabla^2 f(\bm z) \bm x 
        &= \eta \sum_{i=1}^n (\bm \alpha_i \cdot \bm x)^2 p_i(\bm z)
        + \eta (\bm x \cdot \nabla f(\bm z))^2 \\
        &\leq U^2 \eta \sum_{i=1}^n \| \bm x \|_1^2 p_i(\bm z)
        + U^2 \eta \| \bm x \|_1^2 
        = U^2 \eta \| \bm x \|_1^2 + U^2 \eta \| \bm x \|_1^2
        = 2 U^2 \eta \| \bm x \|_1^2,
    \end{align*}
    where the inequality holds from the Cauchy-Schwarz inequality. 
    By Taylor's theorem, for all $\bm x, \bm y \in \mathbb R_+^d$, 
    there exists $\bm z = (1 - \lambda) \bm x + \lambda \bm y$ 
    with $\lambda \in [0, 1]$ such that 
    \begin{align*}
        f(\bm y)
        &= f(\bm x) + \nabla f(\bm x) \cdot (\bm y - \bm x)
        + \frac 1 2 (\bm y - \bm x)^\top \nabla^2f(\bm z)(\bm y - \bm x) \\
        &\leq f(\bm x) + \nabla f(\bm x) \cdot (\bm y - \bm x)
        + \frac 1 2 2U^2 \eta \|\bm y - \bm x \|_1^2.
    \end{align*}

    Now, we turn to prove the smoothness of $\Theta$.
    Recall that the definition of $\Theta$ is
    \begin{align*}
        \Theta(\bm w, \bm \beta)
        = - \frac 1 \eta \ln \frac 1 m
        \sum_{i=1}^{m} \exp
        \left[
            - \eta \left(
                \sign(P_i) \sum_{j \in \Phi(P_i)} w_j
                + \sum_{e \in P_i} \beta_e
            \right)
        \right] 
        - \frac{1}{\nu m} \sum_{e \in E} m_e \beta_e.
    \end{align*}
    Define
    \begin{itemize}
        \item $\bm x := (\bm w, \bm \beta) \in \mathbb R_+^{(n+1) + |E|}$,
        \item $\bm \alpha_i := (\bm a_i, \bm b_i) \in [-2, 2]^{(n+1) + |E|}$, 
        where
        \begin{align*}
            \bm a_i &:= 2 \sign(P_i) \left(
                I(j \in \Phi(P_i))
            \right)_{j=1}^{n+1} \\
            \bm b_i &:= \left( I(e \in P_i) \right)_{e \in E}
        \end{align*}
        and $I(A)$ is the indicator function that returns $1$ if $A$ is true,
        and $0$ otherwise.
        \item $\bm c = (\bm 0, m_{e_1}, m_{e_2}, \dots, m_{e_{|E|}}) \in \mathbb R_+^{(n+1) + |E|}$.
    \end{itemize}
    With these notations, we can rewrite $\Theta$ as
    \begin{align*}
        \Theta(\bm x) =
        - \frac 1 \eta \ln \frac 1 m \sum_{i=1}^m
        e^{- \eta (\bm w_i \cdot \bm x - 1)}
        - \frac{1}{\nu m} \bm c \cdot \bm x
    \end{align*}
    Therefore, we can say that $-\Theta$ is $8\eta$-smooth w.r.t.
    $\ell_1$-norm.
\end{proof}

\subsection{Gradient computation}
The partial differentiates of $\Theta$ is 
\begin{align*}
    \frac{\partial \Theta(\bm w, \bm \beta)}{\partial w_j}
         &= \sum_{P \in \mathcal P_{G^+}} I[j \in \Phi(P)] q(P)
         - \sum_{P \in \mathcal P_{G^-}} I[j \in \Phi(P)] q(P), \\
    \frac{\partial \Theta(\bm w, \bm \beta)}{\partial \beta_e}
         &= \sum_{P \in \mathcal P_{G}} I[e \in P] q(P)
         - \frac{m_e}{\nu m},
\end{align*}
where
\begin{align}
    \label{eq:appendix_path_weight}
    q(P) = \frac{
        \exp\left[
            - \eta \sum_{e \in P}
            (\beta_e + \sign(P) \sum_{j \in \Phi(e)} w_j)
        \right]
    }{
        \sum_{P' \in \mathcal P_{G}}\exp\left[
            - \eta \sum_{e \in P'}
            (\beta_e + \sign(P') \sum_{j \in \Phi(e)} w_j)
        \right]
    }
\end{align}
is the weight on the path $P \in \mathcal P_{G}$.
We can compute (\ref{eq:appendix_path_weight}) by dynamic programming and 
the weight pushing algorithm, proposed by~\cite{mohri+:eurospeech01}.
Therefore, we can compute the gradient vector by dynamic programming.
