# Supplementary material for: Extended Formulations via Decision Diagrams
Source: arXiv:2211.06065 source file (2023-09-06)
Supplement: Supplementary file 4 [file appendix_lpdual.tex]

\section{Derivation of the dual problem of (\ref{prob:zdd_softmargin_primal2})}
The Lagrangian function $L$ of problem (\ref{prob:zdd_softmargin_primal2}) is given as
\begin{align*}
    L(\vecw,\vecs,\vecbeta,\vecd,\gamma,\veclambda,\vectau) =& 
    -\rho + \frac{1}{\nu m}\sum_{e \in E}m_e\beta_e 
    + \sum_{e \in E}d_e (s_{e.v} - s_{e.u} -\sign(e)\sum_{j\in \Phi(e)}w_j -\beta_e)\\
    &
    +\gamma(\sum_{j \in [n]}w_j -w_{n+1}-1) -\sum_{j\in [n]}\lambda_j w_j 
    +\lambda_{n+1}w_{n+1}- \sum_{e}\tau_e \beta_e.
\end{align*}
Taking the partial derivatives, we have
\begin{align*}
    \frac{\partial L}{\partial w_j}
    &= -\sum_{e: j\in \Phi(e)}\sign(e)d_e + \gamma  -\lambda_j \quad (j\in [n]),\\ 
    \frac{\partial L}{\partial w_{n+1}}
    &= -\sum_{e: n+1 \in \Phi(e)}\sign(e)d_e - \gamma  +\lambda_j, \\ 
    \frac{\partial L}{\partial s_v}
    &= \sum_{e:e.v=v}d_e -\sum_{e:e.u=v}d_e \quad (v \in V\setminus \{root,leaf\}),\\
    \frac{\partial L}{\partial \beta_e}
    &= \frac{m_e}{\nu m} - d_e -\tau_e, \text{and} \\
    \frac{\partial L}{\partial \rho}
    &= -1 + \sum_{e: e.v=leaf}d_e.
\end{align*}
Then, by enforncing these partial derivatives to be zero, 
the dual problem is given as 
\begin{align*}
    \max_{\vecd \in [0,1]^{|E|}}& \quad -\gamma  \\ \nonumber
   \text{sub. to:}
    \quad& \sign(j)\sum_{e: j\in\Phi(e)}\sign(e)d_e \leq \gamma \quad (j \in [n+1])\\ 
    \quad& \sum_{e: e.u=u}d_e = \sum_{e: e.v=u} \quad (u \in V\setminus \{root, leaf\}) \\ 
    \quad& \sum_{e, e.u=root}d_e =1, \sum_{e, e.v=leaf}d_e =1, \\ 
    \quad&  0 \leq d_e \leq \frac{m_e}{\nu m} \quad (e \in E).
\end{align*}
