# Supplementary material for: Extended Formulations via Decision Diagrams
Source: arXiv:2211.06065 source file (2023-09-06)
Supplement: Supplementary file 7 [file intro.tex]

\section{Introduction}
\label{sec:intro}
Most tasks in machine learning are formulated as optimization problems.
The amount of data we face in real-world applications
has been rapidly growing, and thus time/memory-efficient optimization
techniques are more in demand than ever.
Various approaches have been proposed to efficiently solve
optimization problems over huge data,
e.g., stochastic gradient descent methods (e.g.,\cite{duchi-etal:jmlr11})
and concurrent computing techniques using GPUs
(e.g.,\cite{raina-etal:icml09}).
Among them, we focus on the ``computation on compressed data'' approach,
where we first compress the given data somehow 
and then employ an algorithm that works directly on the compressed data
(i.e., without decompressing the data) to complete the task, in an
attempt to reduce computation time and/or space.
Algorithms on compressed data are mainly studied 
in string processing (e.g., 
~\cite{rytter:icalp04,lohrey:groups12,lifshits:cpm07,hermelin-etal:stacs09,goto-etal:jda13}),
enumeration of combinatorial objects(e.g.,~\cite{minato:ieice17}),
and combinatorial optimization(e.g.,~\cite{bergman-etal:book16}).
In particular, in the work on combinatorial optimization,
they compress the set of feasible solutions that satisfy given constraints
into a decision diagram so that minimizing a linear objective
can be done by finding the shortest path in the decision diagram.
Although we can find the optimal solution very efficiently when
the size of the decision diagram is small, the method can only be applied to
the case where the feasible solution set is finite and the objective
function is linear.

On the other hand, we mainly consider a more general form of
optimization problems that include
linear constraints with binary coefficients:
% \begin{align}\label{prob:lin_const_opt}
%     \min_{\vecz\in Z \subset \Real^n}& \quad f(\vecz) 
%     \quad \text{s.t.} \quad \matA \vecz \geq \vecb,
%      \quad \matA \in \{0,1\}^{m\times n},~\vecb \in \{0,1\}^m.
% \end{align}
\begin{equation}\label{prob:lin_const_opt}
    \min_{\vecz\in Z \subset \Real^n} f(\vecz)
    \quad \text{s.t.} \quad \matA \vecz \geq \vecb
\end{equation}
for some $\matA \in \{0,1\}^{m\times n}$ and $\vecb \in \{0,1\}^m$,
where $Z$ denotes the constraints other than $\matA \vecz \geq \vecb$.
For example, 0-1 integer programming problems can be formulated
with $Z = \{0,1\}^n$.
In addition, we give a reduction from any optimization problem
with \emph{integer} matrix $\matA$ to a problem (\ref{prob:lin_const_opt}).
So our target problem is fairly general.

Note that even when $Z = \Real^n$ or $Z = \{0,1\}^n$,
we have many applications that fall into (\ref{prob:lin_const_opt}).
\begin{description}
\item[MIP/LP/QP/SDP] 
    Natural integer programming formulations of
	set cover, vertex cover, uncapacitated facility location, 
    prize-collecting Steiner tree, and MAX-SAT problems
	(see, e.g.,\cite{williamson-shmoys:book11}) 
    are of the form of (\ref{prob:lin_const_opt}) with
	linear objective functions. 
    Also, many classes of optimization problems with linear constraints of 0-1 integer coefficients, 
    e.g., LP, QP, SDP 
    (when $Z$ represents positive semi-definite constraints) and MIP, 
    have the form of (\ref{prob:lin_const_opt}).

\item[Hard margin optimization]
    Hard margin optimization with $2$-norm regularization, 
    i.e., SVMs (e.g., \cite{mohri-etal:book18}) or with
	$1$-norm regularization~\cite{demiriz-etal:ml02} 
    are standard formulations for learning classifiers.
    In particular, when the instance space is $\{0,1\}^n$,
    which arises in the bag-of-words or the decision stump
	feature extractions, it is not hard to see that the 
	hard margin optimization falls into 
	(\ref{prob:lin_const_opt}) except that
	$\matA \in \{-1,0,1\}^{m \times n}$, where $m$ is the size of
	the given sample.
	Using our reduction, the problem finally falls into
	(\ref{prob:lin_const_opt}) with a larger value of $n$.
\end{description} 

Without loss of generality, we assume $m > n$ and we are particularly
interested in the case where $m$ is huge.

In this paper, we propose a general algorithm that, when given
a 0-1 constraint matrix
$(\matA,\vecb) \in \{0,1\}^{m \times n} \times \{0,1\}^m$
of an optimization problem (\ref{prob:lin_const_opt}),
produces a matrix
$(\matA',\vecb') \in \{-1,0,1\}^{m' \times (n+n')} \times \{0,1\}^{m'}$
that represents its extended formulation, that is, it holds that
\[
	\exists \vecs \in \Real^{n'},
		\matA' \begin{bmatrix}
			\vecz \\ \vecs
		\end{bmatrix}
		\geq \vecb'  \Leftrightarrow \matA \vecz \geq \vecb
\]
for some $n'$ and $m'$, with the hope that
the size of $(\matA',\vecb')$ is much smaller than that of
$(\matA,\vecb)$ even at the cost of adding $n'$ extra dimensions.
Using the extended formulation, we obtain an equivalent
optimization problem to (\ref{prob:lin_const_opt}):
\begin{equation}\label{prob:zdd_const_opt1}
    \min_{\vecz\in Z \subset \Real^n,\vecs\in \Real^{n'}} f(\vecz) 
	\quad \text{s.t.} \quad
	\matA' 
    \begin{bmatrix}
        \vecz \\ \vecs
    \end{bmatrix}
     \geq \vecb'.
\end{equation}
Then, we can apply existing solvers, e.g., MIP or LP solvers if
$f$ is linear, to (\ref{prob:zdd_const_opt1}), which may significantly
reduce the computation time/space than applying them to the original
problem (\ref{prob:lin_const_opt}).

To obtain a matrix $(\matA',\vecb')$, we first construct
a variant of a decision diagram called a
Non-Deterministic Zero-Suppressed Decision Diagram
(NZDD, for short)~\cite{fujita-etal:tcs20} that somehow represents the 
matrix $(\matA,\vecb)$.
Observing that the constraint $\matA \vecz \geq \vecb$ can be
restated in terms of the NZDD constructed as
``every path length is lower bounded by 0''
for an appropriate edge weighting, we establish the extended formulation
$(\matA',\vecb') \in \{-1,0,1\}^{m' \times (n+n')} \times \{0,1\}^{m'}$
with $m' = |E|$ and $n' = |V|$, where
$V$ and $E$ are the sets of vertices and edges of the NZDD, respectively.
One of the advantages of the result is that 
the size of the resulting optimization problem depends only on the size of
the NZDD and the number $n$ of variables, but
\emph{not} on the number $m$ of the constraints in the original problem. 
Therefore, if the matrix $(\matA,\vecb)$ is well compressed into
a small NZDD, then we obtain an equivalent but concise optimization
problem (\ref{prob:zdd_const_opt1}).

Now we consider the $1$-norm regularized soft margin optimization
as a non-trivial application of our method.
Assume that we are given a sample of size $m$ over the binary
domain $\{0,1\}^n$.
Since the soft margin optimization is also formulated as a linear
programming problem of the form of (\ref{prob:lin_const_opt}),
we could apply our method in a straightforward way as we stated for
the hard margin optimization.
Unfortunately, however, the constraint matrix $(\matA,\vecb)$
for the soft margin optimization is roughly of size $m \times (m+n)$,
and hence our method does not work effectively.
This is because in the LP formulation we have $m$ slack variables,
each of which is associated with an instance-label pair in the sample.
In this paper, we propose a new LP formulation for the soft margin
optimization, which is our second contribution.
We use the same NZDD $(V,E)$ as the one constructed for the hard margin
optimization. Then we introduce a slack variable associated with
each edge of the NZDD to form a constraint matrix
$(\matA',\vecb')$ of size $|E| \times (n+|V|+|E|)$, which is
permissible.
Although our formulation is not equivalent to the standard one for
the soft margin optimization, we show that our feasible solution set is
a subset of that for the standard formulation. This implies that
the margin theory for generalization bound still applies for the solution
of our formulation.
Furthermore, to solve the LP problem obtained, we examine
two specific algorithms besides the standard LP solver.
The first one is based on the column generation
approach~\cite{desaulniers-etal:book05,demiriz-etal:ml02}. 
Although it often performs fast in practice,
no non-trivial iteration bound is known.
The second algorithm we develop is a modification of the
Entropy Regularized LPBoost
(ERLPBoost for short, \cite{warmuth-etal:alt08}) adapted to our
formulation.
We show that the ERLPBoost has the iteration bound of
$O(d^2/\eps^2)$, where $d$ is the depth of the NZDD.

Finally, to realize succinct extended formulations,
we propose practical heuristics for constructing NZDDs,
which is our third contribution.
Since it is not known to construct an NZDD of small size,
we first construct a ZDD of minimal size, where the ZDD is a restricted
form of the NZDD representation. To this end, we use a ZDD compression
software called \texttt{zcomp}~\cite{toda:ds13}.
Then, we give rewriting rules for NZDDs that reduce both the numbers of vertices
and edges, and apply them to obtain NZDDs of smaller size of
$V$ and $E$.
Although the rules may increase the size of NZDDs
(i.e., the total number of edge labels), the rules seem to work
effectively since reducing $|V|$ and $|E|$ is more important
for our purpose.

Experimental results on synthetic and real data sets show that 
our algorithms improve time/space efficiency significantly, especially when 
$m \gg n$, where the datasets tend to have concise NZDD representations.
